# Supplementary material for: Adaptive Dropout: Unleashing Dropout across Layers for Generalizable Image Super-Resolution
Source: arXiv:2506.12738 source file (2025-06-15)
Supplement: Supplementary file 1 [file suppl.tex]

\clearpage
\setcounter{page}{1}
\setcounter{figure}{0}
\setcounter{table}{0}
\maketitlesupplementary

\setcounter{section}{0}

\section{More Implementation Details}
\label{sec:details}
\subsection{Dataset details}
We train our blind SR model on the DIV2K dataset, cropping the high-resolution images into smaller $800\times800$ images to reduce the network's computational burden. To degrade the high-resolution images into corresponding low-resolution images, we use a widely employed multi-degradation setting. Our training degradation setup remains consistent with baseline methods, using a "second-order" degradation generation setting. In each order, the image has a certain probability of sequentially applying noise, blur, and JPEG degradation types during downsampling to disrupt the original image information maximally.

To test the generalization ability of blind SR models trained on the multi-degradation setting, we adopt the five widely used datasets Set5, Set14, BSD100, Manga109, and Urban100. Different from training degradations, we simply degrade the HR images from these datasets with eight types of synthetic degradations or degradation combinations, including bicubic (abbreviated as clean), bicubic + blur (abbreviated as blur), bicubic + noise (abbreviated as noise), bicubic + jpeg (abbreviated as jpeg), bicubic + blur + noise (abbreviated as b+n), bicubic + blur + jpeg (abbreviated as b+j), bicubic + noise + jpeg (abbreviated as n+j), bicubic + blur + noise + jpeg (abbreviated as b+n+j), where bicubic is bicubic downsampling, b is \textit{blur}, n is \textit{noise}, j is \textit{jpeg}. These degradations include those similar to the training degradations (such as b+n+j) and those far from the training degradations (such as clean, noise). Therefore, these eight degradation types can effectively illustrate the fitting and generalization capabilities of a blind SR model. However, it is important to note that the above method of evaluating the capabilities of blind SR models is only valid on synthetic datasets. Considering that the ultimate goal of blind SR models is to effectively enhance the quality and resolution of photographs in the real world, we also employ several real-world datasets. RealSR and DRealSR are two recent real-world super-resolution datasets, where the low-resolution and high-resolution images are captured by cameras at different focal lengths, which better reflect the capabilities of blind SR models in the real world compared to synthetic datasets. Additionally, to remain consistent with baseline methods, we also use the realistic NTIRE 2018 SR challenge data to demonstrate the generalization capabilities of our method.

\subsection{Training details}
During the training process, we employ the L1 loss function and the Adam optimizer. The values of $\beta_1$ and $\beta_2$ of the Adam optimizer are set to 0.9 and 0.999 respectively. The batch size is set to 16, and the low-resolution (LR) images have dimensions of 32×32 pixels. We implement a cosine annealing learning strategy to adjust the learning rate. Initially, the learning rate is set to $2 \times 10^{-4}$. The cosine annealing period for adjusting the learning rate spans 500,000 iterations. We train and test all our models using the PyTorch framework and conducted the training on 3090 GPUs.
\subsection{Metrics}
We primarily use PSNR(Peak Signal-to-Noise Ratio) to measure the performance of the model on different datasets. For real-world datasets, we also use LPIPS(Learned Perceptual Image Patch Similarity) to evaluate the perceptual quality of the restored high-resolution images, which is more important for real-world images. We present the relevant LPIPS results in the supplementary materials.
\section{Detailed Comparisons}
\label{sec:comparison}
We show detailed comparison data with Simple-Align in~\tablename~\ref{tab:suppl_comparison}. We outperform Simple-Align on almost all degradations. The result is understandable for we consider the importance of explicit generalization for intermediate layers. We show more visual results of SRResNet with different regularization methods in~\figurename~\ref{fig:suppl_comparison_1},~\figurename~\ref{fig:suppl_comparison_2},~\figurename~\ref{fig:suppl_comparison_3}, and~\figurename~\ref{fig:suppl_comparison_4}.
\begin{table}[h]
    \centering
    \small
  \setlength{\abovecaptionskip}{-0pt}
	\setlength{\belowcaptionskip}{-4pt}
	
     \caption{\textbf{The performance of SRResNet on Set5 and Set14 with different annealing strategies.} These annealing strategies are all for Explicit Adaptive Dropout and are explicitly adopted.}
     \label{tab:strategy}
    \begin{tabular}{cccc}
    \hline
         \multirow{2}{*}{dropout~format} &\multirow{2}{*}{training~strategy}  &\multicolumn{2}{c}{psnr} \\
         ~ & &Set5 &Set14 \\ \hline
         \multirow{4}{*}{standard dropout} &None &24.33 &22.45\\
         ~ &linear annealing &24.55 &22.83 \\
         ~ &layer-wise annealing &\textbf{24.89} &\textbf{23.01} \\
         ~ &linear+layer-wise &24.81 &22.94 \\ \hline
         \multirow{4}{*}{adaptive dropout} &None &25.89 &23.36\\
         ~ &linear annealing &25.85 &23.26\\
         ~ &layer-wise annealing &\textbf{26.07} &\textbf{23.46}\\
         ~ &linear+layer-wise &25.91 &23.32 \\ \hline
    \end{tabular}
    \vskip -0.10cm
\end{table}

\begin{figure*}[t]
	\centering
	\includegraphics[width=1\linewidth]{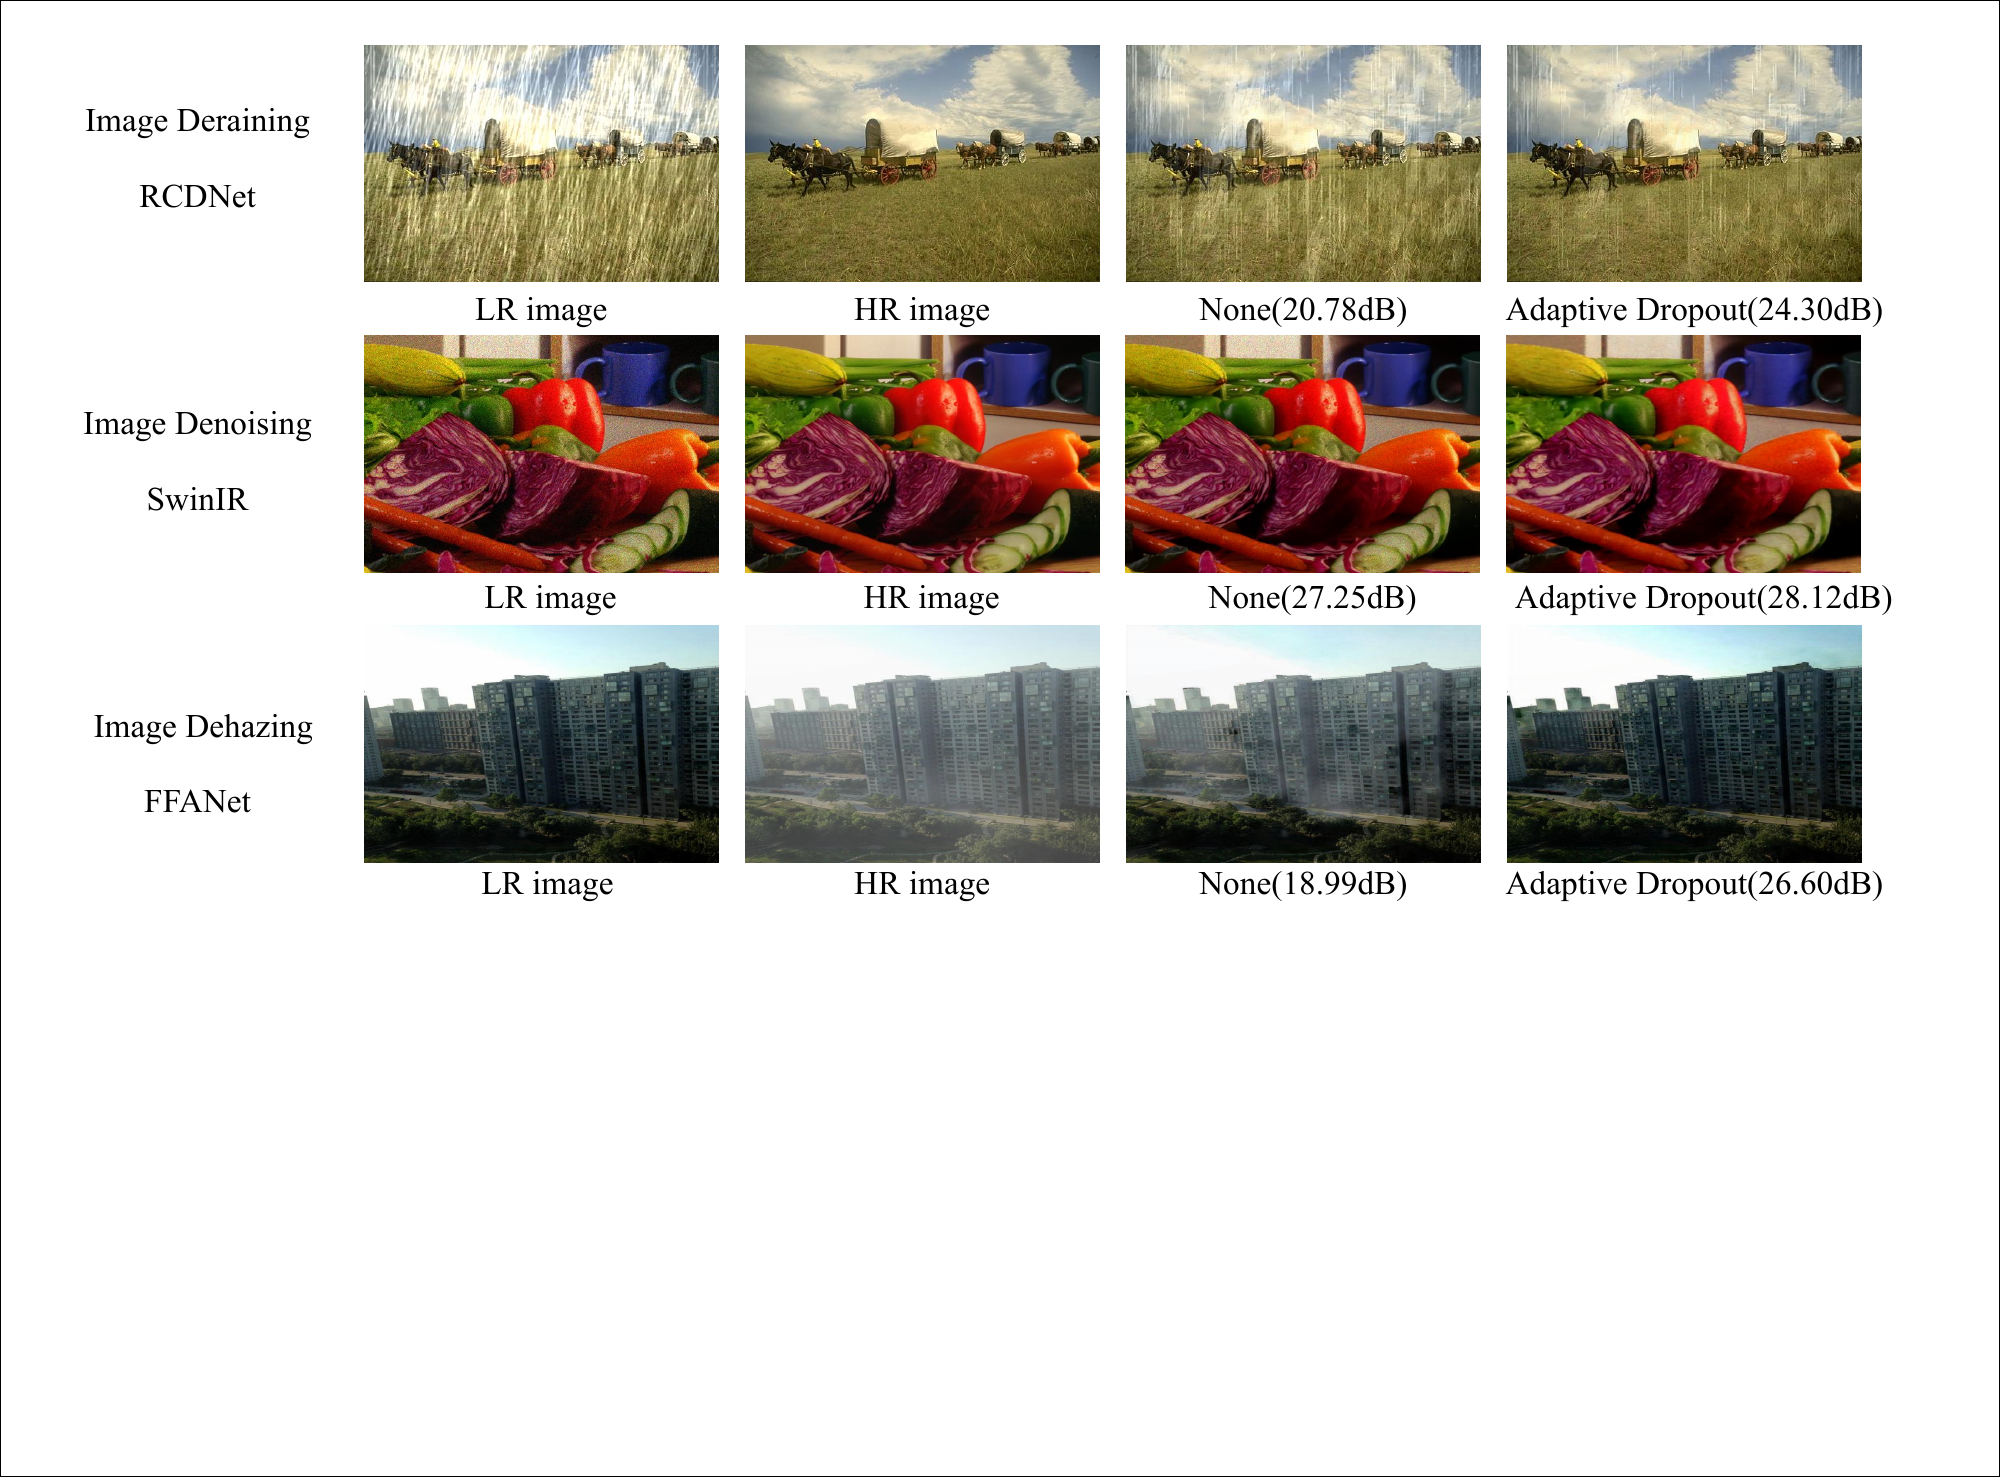}
    \vspace{-5mm}
	\caption{ \textbf{Visual comparison of baseline w or w/o our regularization methods in single-degradation tasks.}}
	\label{fig:single}
\end{figure*}

\begin{figure}[t]
	\centering
	\includegraphics[width=1\linewidth]{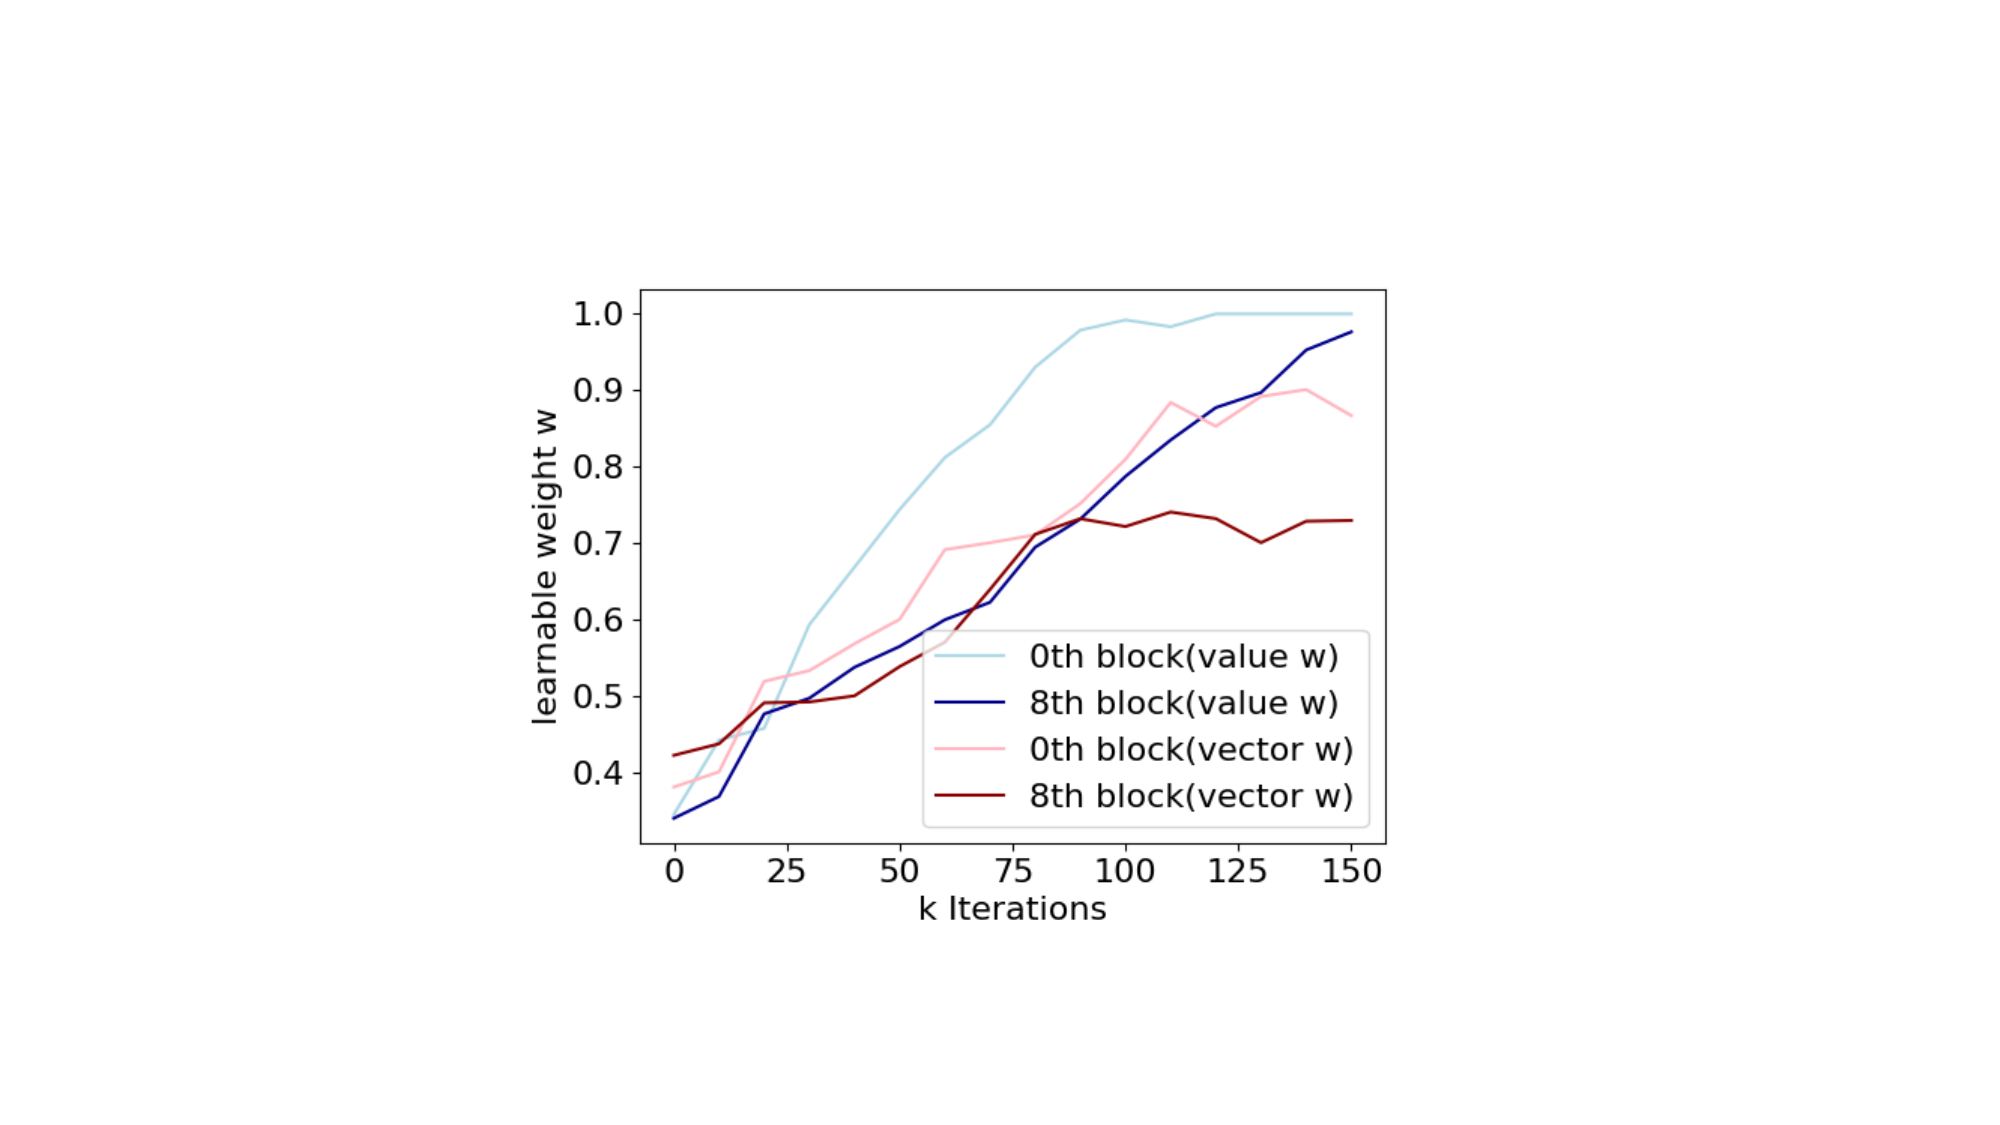}
    \vspace{-5mm}
	\caption{ \textbf{The trend of the average value of vector w and value w over the training process.} Vector w is more difficult to converge to 1 compared to value w.}
	\label{fig:format}
\end{figure}

\begin{table*}[h]
    \centering
    \small
  \setlength{\abovecaptionskip}{-0pt}
	\setlength{\belowcaptionskip}{-4pt}
	
     \caption{\textbf{The performance of SRResNet with different formats of $w$.} $nth~block$ means that before $nth$ block, we use $value~w$ and after $nth$ block, we use $vector~w$.}
     \label{tab:w_format}
    \begin{tabular}{ccccccc}
    \hline
         \multirow{2}{*}{nth block} &\multicolumn{6}{c}{model performance} \\
         ~ &Set5 &Set14 &BSD100 &Manga109 &Urban100 &average\\ \hline
         0 &24.61 &22.55 &23.00 &19.13 &20.67 &21.99\\
         4 &24.58 &22.56 &22.94 &19.23 &20.69 &22.00\\
         8 &24.55 &22.50 &22.94 &19.29 &20.81 &\textbf{22.09}\\
         12 &24.37 &22.40 &22.75 &19.40 &20.78 &21.94\\
         16 &24.28 &22.36 &22.86 &19.44 &21.02 &21.98\\ \hline
    \end{tabular}
    \vskip -0.10cm
\end{table*}

\section{More discussions}
\label{sec:discussion}
\subsection{About the annealing strategy for Explicit Adaptive Dropout}
For Explicit Adaptive Dropout, we use a layer-wise annealing strategy as the adaptive training strategy to help blind SR models generalize better. A competing annealing strategy involves reducing the weighted dropout $w$ by the same amount in every layer at regular intervals until $w$ reaches $0$. However, we found that this strategy does not account for the different levels of sensitivity to perturbations between shallow and deep layers of the network, resulting in poor generalization. Additionally, we also attempt to gradually reduce the $w$ corresponding to the block being annealed while performing layer-wise annealing. Specifically, originally during layer-wise annealing, we keep $w$ constant until $t$ iterations, after which we set the $w$ for that block to $1$. Now, we linearly decrease $w$ to 0 over these $t$ iterations. We find that although this fully follows the pattern we discover in the learnable weighted structure, it does not improve the model's generalization capability and performs slightly worse than simple layer-wise annealing.  This indicates that when adding regularization to the intermediate layers of the network, it is more important to consider the different requirements of each layer for regularization. For the learnable weighted structure, gradually reducing $w$ to $1$ primarily satisfies the need for the network to fit the training set, which may not necessarily have a positive impact on generalization performance. Therefore, when testing our two designed variants on the blind SR model, we often find that the explicit weighted dropout outperforms the implicit weighted dropout. This suggests that gradually reducing $w$ to $1$ is not essential; what is more important is the relative relationship of $w$ between different layers. We show the performance of SRResNet on Set5 and Set14 with different training strategies in~\tablename~\ref{tab:strategy}.

\begin{table}[h]
    \centering
    \small
  \setlength{\abovecaptionskip}{-0pt}
	\setlength{\belowcaptionskip}{-4pt}
	
     \caption{\textbf{The average performance of SRResNet on the five synthetic datasets.} We only calculate the average on the first four degradations(clean, noise, blur, jpeg), considering they best reflect the network's generalization capability. $plan~A$ is using $value~w$ for shallow layers and using $vector~w$ for deep layers. $plan~B$ is the opposite one.}
     \label{tab:w_position}
    \begin{tabular}{ccccccc}
    \hline
         postion &average performance \\ \hline
         plan A &\textbf{22.09} \\
         plan B &22.01 \\ \hline
    \end{tabular}
    \vskip -0.10cm
\end{table}

\subsection{About vector w and value w}
For Implicit Adaptive Dropout, we use different formats of w for different layers. Specifically, we use \texttt{value w} for shallow layers and \texttt{vector w} for deep layers. Here, we explain the specific reasons. For \texttt{vector w}, we plot the average value of w corresponding to that layer over the training process as a curve and display it alongside the w for \texttt{value w} in~\figurename~\ref{fig:format}. Compared to \texttt{value w}, the average value of \texttt{vector w} is harder to converge. This indicates that this perturbation is stronger and affects the generalization of specific degradations. The perturbation given by \texttt{value w} is weaker and affects more general generalization. If the perturbation in shallow layers is too strong, it can affect the stability of network training. Therefore, we use \texttt{value w} in shallow layers and \texttt{vector w} in deep layers, achieving a good trade-off between fitting and generalization.

Furthermore, we conduct ablation experiments to determine from which layer to switch from \texttt{value w} to \texttt{vector w} and show the result in~\tablename~\ref{tab:w_format}. It can be observed that using only \texttt{vector w} or \texttt{value w} alone cannot perform well across all datasets. Combining both achieves a better balance in different scenarios. Specifically, using \texttt{vector w} allows for the allocation of appropriate $w$ to different features, better addressing the imbalance between channels, thereby forming a more robust general representation that is not only applicable to different degradations but also to different scenes. Using \texttt{value w} reduces the network parameters for learning $w$, with all channels sharing one $w$. While this is not conducive to alleviating the imbalance between channels, it ensures the network's fitting ability, which to some extent is a result of this imbalance. Manga100 and Urban100 datasets in the test set have distributions significantly different from the training set, so \texttt{vector w} performs better on these datasets. Conversely, the Set5, Set14, and BSD100 datasets are relatively close to the training set, and using \texttt{value w} may to some extent help restore image quality in these datasets. Therefore, we combine both, using them at different layers, to achieve good generalization performance across all datasets. We decide to switch from \texttt{value w} to \texttt{vector w} at the midpoint of the network, which exhibits the best performance as shown in~\tablename~\ref{tab:w_format}. Additionally, we conduct ablation experiments on whether to use \texttt{value w} or \texttt{vector w} in shallow or deep layers in~\tablename~\ref{tab:w_position}, which demonstrate that using \texttt{value w} in shallow layers and \texttt{vector w} in deep layers can lead to better generalization performance.

\begin{figure}[t]
\centering
\includegraphics[width=1\linewidth]{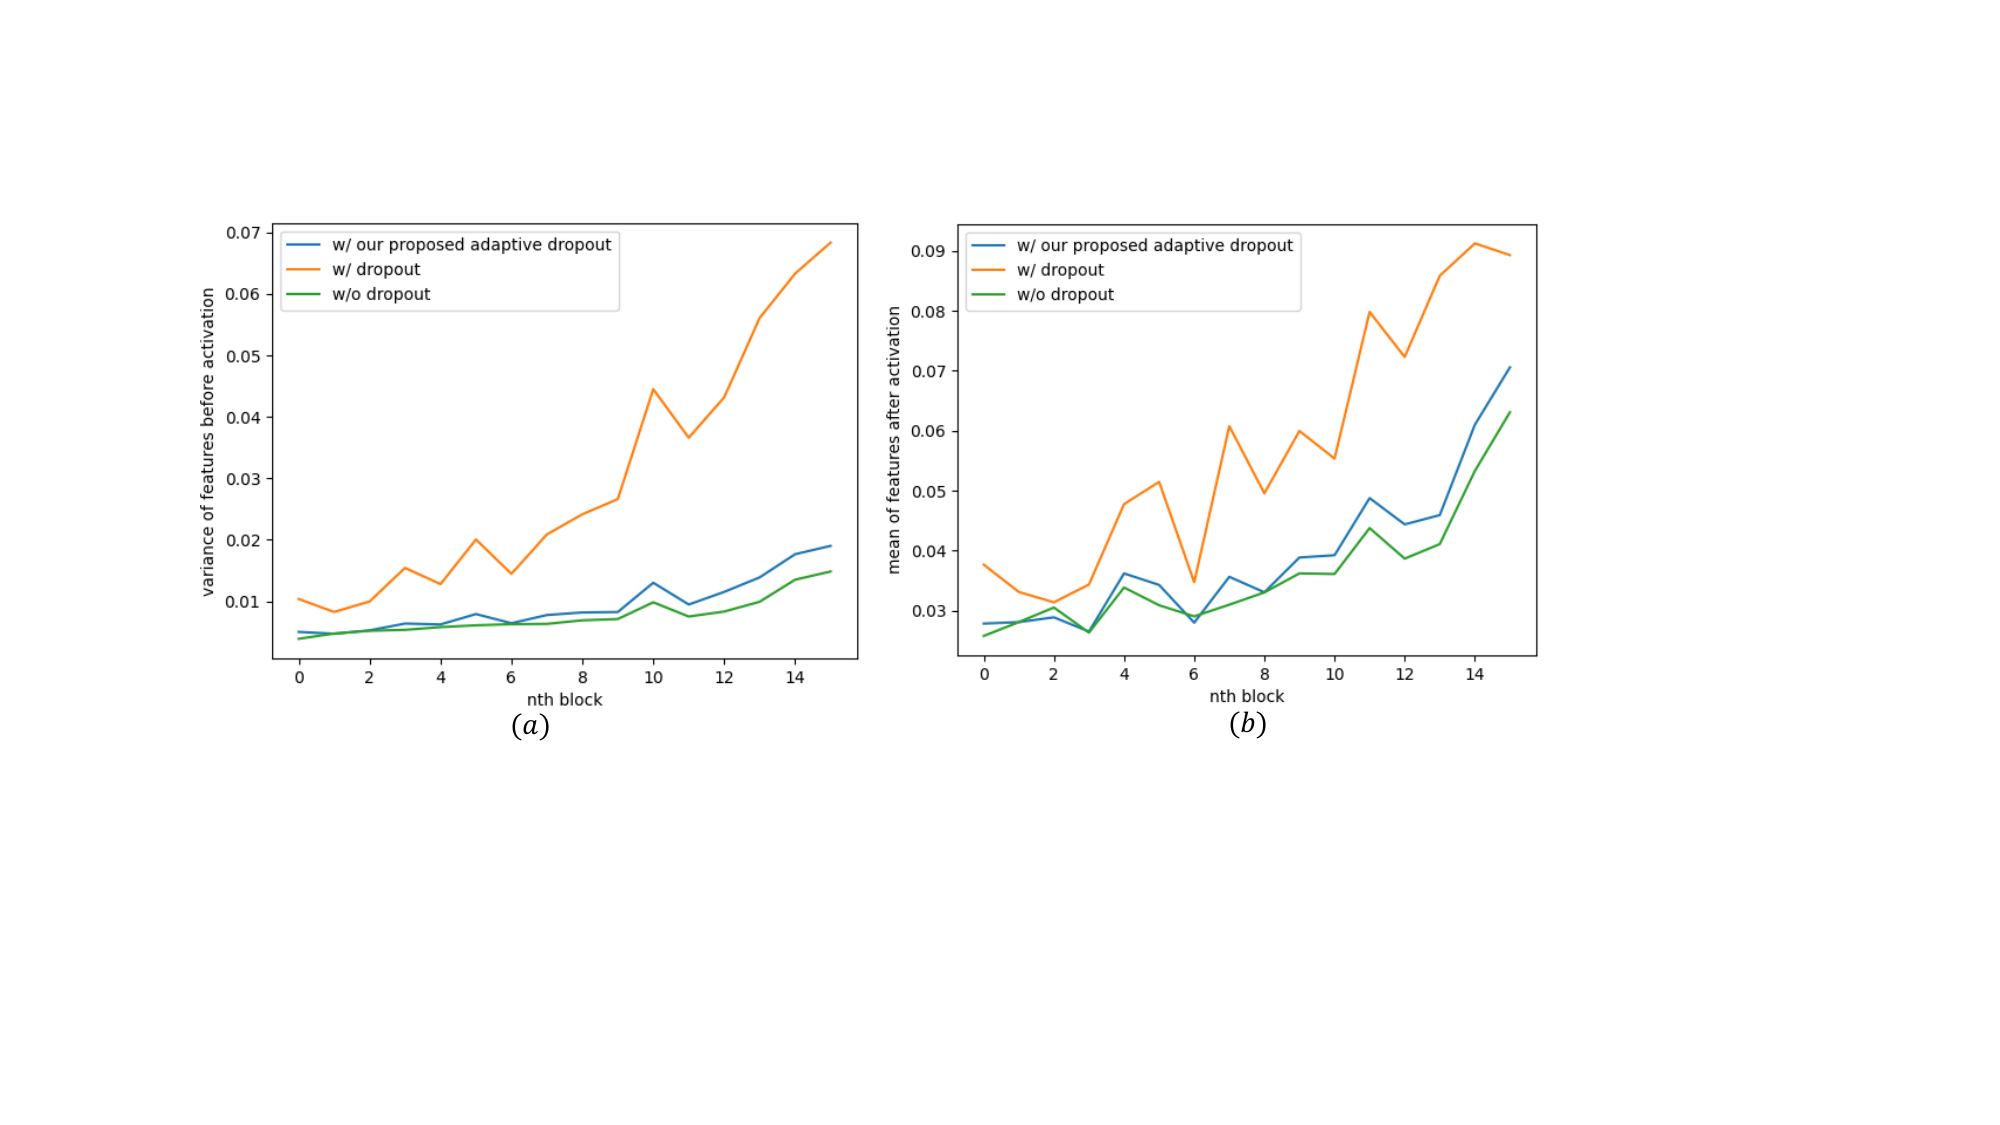}
\vspace{-4mm}
\caption{\textbf{statistics of features with or without dropout during training.} (a) shows that dropout alters the variance of features although it keeps the mean. (b) shows that the mean of features also changes after activation when they undergo dropout before.}
\label{fig:statistic}
\vspace{-4mm}
\end{figure}

\subsection{About the inconsistency during training}
 As illustrated in section 3.1 of \citet{li2019understanding} or section 2.1 of \citet{kim2023use}, the variance of features has been altered after dropout during training. And then after non-linear activation functions, the variance shift leads to the mean shift. We also provide the statistical changes in features during training in Fig. \ref{fig:statistic}, which can be alleviated with our proposed adaptive dropout.
 
\subsection{About the relationship between the two variants}
For Adaptive Dropout, we design two variants based on how they adopt the adaptive training strategy. Through experimental results, it can be observed that the two variants exhibit different performances across various degradations and datasets. The biggest difference between the two variants lies in the different ways they utilize the adaptive training strategy. On the basis of layer-wise annealing, Explicit adaptive dropout explicitly employs this strategy, maintaining $w$ constant before annealing to provide greater perturbation to intermediate layer features. In contrast, Implicit Adaptive Dropout implicitly utilizes this strategy while striving to ensure the network's fitting ability.

Additionally, there is also room for combining these two variants. In Implicit Adaptive Dropout, we also observe similar annealing phenomena as in~\figurename~\ref{fig:format}. However, directly combining the two variants is somewhat challenging, so we will explore this in future work, where explicit annealing in shallow layers and implicit annealing in deep layers may be an area worth exploring.

\begin{table*}[t]
  \small
  \setlength{\abovecaptionskip}{-2pt}
	\setlength{\belowcaptionskip}{-4pt}
	
  \begin{center}
    \caption{\textbf{The PSNR ($\mathbf{dB}$) results of models with $\times 4$.} We test them on eight types of degradations or multi-degradations($b$ is $blur$, $n$ is $noise$, $j$ is $jpeg$). \textbf{\textcolor{red}{Red}} and \underline{\textcolor{blue}{Blue}} indicate the best and the second-best performance, respectively.}
      \label{tab:suppl_comparison}
  \resizebox{\linewidth}{!}{
    \begin{tabular}{|l|c|cc|cc|cc|cc|cc|}
    \hline
        \multirow{2}{*}{Models} &\multirow{2}{*}{Regularization}  & \multicolumn{2}{c|}{Set5~\cite{bevilacqua2012low}} & \multicolumn{2}{c|}{Set14~\cite{yang2010image}} & \multicolumn{2}{c|}{BSD100~\cite{martin2001database}} & \multicolumn{2}{c|}{Manga109~\cite{matsui2017sketch}} &  \multicolumn{2}{c|}{Urban100~\cite{huang2015single}} \\ \cline{3-12}
        &  & \multicolumn{1}{c}{clean} & blur  & \multicolumn{1}{c}{clean} & blur  & \multicolumn{1}{c}{clean} & blur  & \multicolumn{1}{c}{clean} & blur  & \multicolumn{1}{c}{clean} & blur \\ \hline
        \multirow{4}{*}{SRResNet~\cite{ledig2017photo}} & None    & 24.89  & 24.76  & 22.60  & 22.50  & 23.06  & 22.99  & 18.42  & 18.75  & 21.24  & 21.06  \\ 
        ~ & Simple-Align~\cite{wang2024navigating}                   & 25.94  & \underline{\textcolor{blue}{25.45}}  & \underline{\textcolor{blue}{23.46}}  & 23.18  & 23.69  & 23.47  & 19.34  & 19.50  & 21.83  & 21.40  \\ 
        ~ & Explicit Adaptive Dropout & \textbf{\textcolor{red}{26.11}} & \textcolor{black}{25.39} & \textcolor{black}{23.42} & \underline{\textcolor{blue}{23.20}} & \textbf{\textcolor{red}{23.76}} & \textbf{\textcolor{red}{23.59}} & \underline{\textcolor{blue}{19.40}} & \underline{\textcolor{blue}{19.62}} & \underline{\textcolor{blue}{21.87}} & \textbf{\textcolor{red}{21.48}} \\ 
        ~ & Implicit Adaptive Dropout & \underline{\textcolor{blue}{26.09}} & \textbf{\textcolor{red}{25.56}} & \textbf{\textcolor{red}{23.47}} & \textbf{\textcolor{red}{23.21}} & \underline{\textcolor{blue}{23.73}} & \underline{\textcolor{blue}{23.50}} & \textbf{\textcolor{red}{19.51}} & \textbf{\textcolor{red}{19.69}} & \textbf{\textcolor{red}{21.90}} & \underline{\textcolor{blue}{21.40}} \\ \hline
        \multirow{4}{*}{RRDB~\cite{zhang2018image}} & None    & 25.21  & 25.14  & 22.98  & 22.65  & 23.38  & 23.31  & 18.59  & 18.64  & 21.57  & 21.17  \\ 
        ~ & Simple-Align~\cite{wang2024navigating}                   & 26.46  & 26.27  & \underline{\textcolor{blue}{23.76}}  & 23.59  & 23.90  & \underline{\textcolor{blue}{23.94}}  & 19.21  & 19.45  & 22.21  & \textbf{\textcolor{red}{21.94}}  \\ 
        ~ & Explicit Adaptive Dropout & \textbf{\textcolor{red}{26.64}} & \underline{\textcolor{blue}{26.34}} & \textcolor{black}{23.72} & \underline{\textcolor{blue}{23.69}} & \textbf{\textcolor{red}{24.04}} & \textbf{\textcolor{red}{24.02}} & \underline{\textcolor{blue}{19.47}} & \underline{\textcolor{blue}{19.71}} & \underline{\textcolor{blue}{22.23}} & \underline{\textcolor{blue}{21.76}} \\ 
        ~ & Implicit Adaptive Dropout & \underline{\textcolor{blue}{26.57}} & \textbf{\textcolor{red}{26.30}} & \textbf{\textcolor{red}{23.79}} & \textbf{\textcolor{red}{23.76}} & \underline{\textcolor{blue}{24.00}} & \textcolor{black}{23.89} & \textbf{\textcolor{red}{19.53}} & \textbf{\textcolor{red}{19.79}} & \textbf{\textcolor{red}{22.12}} & \textcolor{black}{21.73} \\ \hline
        \multirow{4}{*}{SwinIR~\cite{liang2021swinir}} & None      & 26.25  & 26.03  & 23.76  & \underline{\textcolor{blue}{23.47}}  & 23.91  & \underline{\textcolor{blue}{23.83}}  & 19.10  & 19.19  & 22.18  & 21.90   \\ 
        ~ & Simple-Align~\cite{wang2024navigating}                   & 26.40  & \underline{\textcolor{blue}{26.15}}  & 23.89  & \underline{\textcolor{blue}{23.50}}  & 23.97  & \textbf{\textcolor{red}{23.95}}  & 19.21  & 19.34  & 22.27  & 22.07  \\ 
        ~ & Explicit Adaptive Dropout & \textbf{\textcolor{red}{26.54}} & \textbf{\textcolor{red}{26.21}} & \underline{\textcolor{blue}{23.92}} & \textbf{\textcolor{red}{23.56}} & \textbf{\textcolor{red}{24.09}} & \textcolor{black}{23.59} & \underline{\textcolor{blue}{19.22}} & \underline{\textcolor{blue}{19.39}} & \textbf{\textcolor{red}{22.41}} & \textbf{\textcolor{red}{22.19}} \\ 
        ~ & Implicit Adaptive Dropout & \underline{\textcolor{blue}{26.46}} & \textcolor{black}{26.12} & \textbf{\textcolor{red}{23.95}} & \textcolor{black}{23.41} & \underline{\textcolor{blue}{24.01}} & \textcolor{black}{23.50} & \textbf{\textcolor{red}{19.31}} & \textbf{\textcolor{red}{19.44}} & \underline{\textcolor{blue}{22.32}} & \underline{\textcolor{blue}{22.16}} \\ \hline
        & &  \multicolumn{1}{c}{noise} & jpeg & \multicolumn{1}{c}{noise} & jpeg & \multicolumn{1}{c}{noise} & jpeg & \multicolumn{1}{c}{noise} & jpeg & \multicolumn{1}{c}{noise} & jpeg \\ \hline
        \multirow{4}{*}{SRResNet~\cite{ledig2017photo}} & None    & 22.02  & 23.72  & 20.81  & 21.84  & 20.34  & 22.48  & 19.74  & 18.30  & 19.73  & 20.60  \\ 
        ~ & Simple-Align~\cite{wang2024navigating}                   & 22.32  & 24.33  & 21.11  & 22.45  & 21.46  &22.93   & 18.64  & 19.05  & 19.86  & 21.10  \\ 
        ~ & Explicit Adaptive Dropout & \textbf{\textcolor{red}{22.41}} & \textbf{\textcolor{red}{24.38}} & \underline{\textcolor{blue}{21.14}} & \underline{\textcolor{blue}{22.46}} & \underline{\textcolor{blue}{21.48}} & \textbf{\textcolor{red}{23.00}} & \underline{\textcolor{blue}{18.67}} & \underline{\textcolor{blue}{19.07}} & \textbf{\textcolor{red}{19.90}} & \underline{\textcolor{blue}{21.11}} \\ 
       ~ & Implicit Adaptive Dropout & \textbf{\textcolor{red}{22.41}} & \underline{\textcolor{blue}{24.36}} & \textbf{\textcolor{red}{21.15}} & \textbf{\textcolor{red}{22.51}} & \textbf{\textcolor{red}{21.53}} & \textbf{\textcolor{red}{23.00}} & \textbf{\textcolor{red}{18.76}} & \textbf{\textcolor{red}{19.20}} & \textbf{\textcolor{red}{19.90}} & \textbf{\textcolor{red}{21.15}} \\ \hline
       \multirow{4}{*}{RRDB~\cite{zhang2018image}} & None    & 21.79  & 23.86  & 20.70  & 22.07  &20.98   & 22.73  & 18.29  & 18.44  & 19.61  & 20.92  \\ 
        ~ & Simple-Align~\cite{wang2024navigating}                   & 22.71  & 24.56  & 21.45  & 22.60  & \underline{\textcolor{blue}{21.76}}  & 23.09  &18.78   & 19.08  & \textbf{\textcolor{red}{20.00}}  & \textbf{\textcolor{red}{21.33}}  \\ 
        ~ & Explicit Adaptive Dropout & \textbf{\textcolor{red}{22.80}} & \underline{\textcolor{blue}{24.62}} & \underline{\textcolor{blue}{24.53}} & \underline{\textcolor{blue}{22.67}} & \textbf{\textcolor{red}{21.84}} & \textbf{\textcolor{red}{23.20}} & \underline{\textcolor{blue}{18.84}} & \underline{\textcolor{blue}{19.22}} & \underline{\textcolor{blue}{19.94}} & \underline{\textcolor{blue}{21.24}} \\ 
        ~ & Implicit Adaptive Dropout & \underline{\textcolor{blue}{22.81}} & \textbf{\textcolor{red}{24.59}} & \textbf{\textcolor{red}{21.58}} & \textbf{\textcolor{red}{22.80}} & \underline{\textcolor{blue}{21.71}} & \underline{\textcolor{blue}{23.13}} & \textbf{\textcolor{red}{18.87}} & \textbf{\textcolor{red}{19.23}} & \textcolor{black}{19.87} & \textcolor{black}{21.23} \\ \hline
        \multirow{4}{*}{SwinIR~\cite{liang2021swinir}} & None      & 22.96  & 24.37  & 21.56  & 23.04  & 22.12  & 23.04  & 18.71  & 18.95  & 20.56  & 21.32  \\ 
        ~ & Simple-Align~\cite{wang2024navigating}                   & 23.49  & \underline{\textcolor{blue}{24.62}}  & 21.64  & 23.19  & \underline{\textcolor{blue}{22.21}}  & 23.15  & 18.90  & 19.15  & 20.69  & 21.37  \\ 
        ~ & Explicit Adaptive Dropout & \textbf{\textcolor{red}{23.63}} & \textbf{\textcolor{red}{24.68}} & \underline{\textcolor{blue}{21.67}} & \textbf{\textcolor{red}{23.29}} & \textbf{\textcolor{red}{22.24}} & \textbf{\textcolor{red}{23.29}} & \underline{\textcolor{blue}{18.92}} & \underline{\textcolor{blue}{19.27}} & \textbf{\textcolor{red}{20.85}} & \textbf{\textcolor{red}{21.52}} \\ 
        ~ & Implicit Adaptive Dropout & \underline{\textcolor{blue}{23.49}} & \textcolor{black}{24.49} & \textbf{\textcolor{red}{21.69}} & \underline{\textcolor{blue}{23.19}} & \textcolor{black}{22.19} & \underline{\textcolor{blue}{23.28}} & \textbf{\textcolor{red}{19.02}} & \textbf{\textcolor{red}{19.31}} & \underline{\textcolor{blue}{20.74}} & \underline{\textcolor{blue}{21.40}} \\ \hline
        ~ & ~ & b+n & b+j & b+n & b+j & b+n & b+j & b+n & b+j & b+n & b+j \\ \hline
        \multirow{4}{*}{SRResNet~\cite{ledig2017photo}} & None    & 23.31  & 23.44  & 21.81  & 21.70  & 22.27  & 22.34  & 18.60  & 18.53  & 20.46  & 20.30  \\ 
        ~ & Simple-Align~\cite{wang2024navigating}                   & 23.64  & \textbf{\textcolor{red}{23.85}}  & 22.12  & 22.24  & 22.43  & 22.71  & 19.22  & 19.14  & \underline{\textcolor{blue}{20.56}}  & 20.61  \\ 
        ~ & Explicit Adaptive Dropout & \textbf{\textcolor{red}{23.74}} & \underline{\textcolor{blue}{23.80}} & \textbf{\textcolor{red}{22.15}} & \textbf{\textcolor{red}{22.29}} & \textbf{\textcolor{red}{22.48}} & \textbf{\textcolor{red}{22.81}} & \underline{\textcolor{blue}{19.26}} & \underline{\textcolor{blue}{19.23}} & \textbf{\textcolor{red}{20.57}} & \textbf{\textcolor{red}{20.66}} \\ 
        ~ & Implicit Adaptive Dropout & \underline{\textcolor{blue}{23.65}} & \textcolor{black}{23.73} & \underline{\textcolor{blue}{22.12}} & \textbf{\textcolor{red}{22.29}} & \underline{\textcolor{blue}{22.44}} & \underline{\textcolor{blue}{22.78}} & \textbf{\textcolor{red}{19.51}} & \textbf{\textcolor{red}{19.29}} & \textcolor{black}{20.50} & \underline{\textcolor{blue}{20.63}} \\ \hline
        \multirow{4}{*}{RRDB~\cite{zhang2018image}} & None    & 23.52  & 23.48  & 22.05  & 21.76  & 22.40  & 22.46  & 18.82  & 18.44  & 20.57  & 20.39  \\ 
        ~ & Simple-Align~\cite{wang2024navigating}                   & \underline{\textcolor{blue}{23.80}}  & 23.95  & 22.35  & 22.29  & 22.63  & 22.88  & 19.33  & 19.21  & \textbf{\textcolor{red}{20.68}}  & \underline{\textcolor{blue}{20.79}}  \\ 
        ~ & Explicit Adaptive Dropout & \textbf{\textcolor{red}{23.83}} & \underline{\textcolor{blue}{24.03}} & \underline{\textcolor{blue}{22.38}} & \underline{\textcolor{blue}{22.36}} & \textbf{\textcolor{red}{22.67}} & \textbf{\textcolor{red}{22.93}} & \underline{\textcolor{blue}{19.45}} & \underline{\textcolor{blue}{19.28}} & \underline{\textcolor{blue}{20.66}} & \textbf{\textcolor{red}{20.79}} \\ 
        ~ & Implicit Adaptive Dropout & \textcolor{black}{23.76} & \textbf{\textcolor{red}{24.05}} & \textbf{\textcolor{red}{22.36}} & \textbf{\textcolor{red}{22.41}} & \underline{\textcolor{blue}{22.63}} & \underline{\textcolor{blue}{22.92}} & \textbf{\textcolor{red}{19.48}} & \textbf{\textcolor{red}{19.28}} & \textcolor{black}{20.62} & \textcolor{black}{20.71} \\ \hline
        \multirow{4}{*}{SwinIR~\cite{liang2021swinir}} & None      & 23.80  & 23.84  & 22.20  & 22.26  & 22.61  & 22.82  & 19.07  & 19.02  & 20.89  & 20.79  \\ 
        ~ & Simple-Align~\cite{wang2024navigating}                   & 24.13  & 24.17  & 22.55  & 22.32  & 22.74  & 22.97  & 19.23  & 19.22  & \textbf{\textcolor{red}{21.02}}  & \textbf{\textcolor{red}{20.98}}  \\ 
        ~ & Explicit Adaptive Dropout & \textbf{\textcolor{red}{24.24}} & \underline{\textcolor{blue}{24.27}} & \textbf{\textcolor{red}{22.91}} & \textbf{\textcolor{red}{22.41}} & \textbf{\textcolor{red}{22.81}} & \textbf{\textcolor{red}{23.05}} & \underline{\textcolor{blue}{19.25}} & \underline{\textcolor{blue}{19.29}} & \underline{\textcolor{blue}{21.00}} & \underline{\textcolor{blue}{20.96}} \\ 
        ~ & Implicit Adaptive Dropout & \underline{\textcolor{blue}{24.18}} & \textbf{\textcolor{red}{24.30}} & \underline{\textcolor{blue}{22.78}} & \underline{\textcolor{blue}{22.36}} & \underline{\textcolor{blue}{22.80}} & \textbf{\textcolor{red}{23.05}} & \textbf{\textcolor{red}{19.31}} & \textbf{\textcolor{red}{19.37}} & \textcolor{black}{20.92} & \textcolor{black}{20.94} \\ \hline
        ~ & ~ & n+j & b+n+j & n+j & b+n+j & n+j & b+n+j & n+j & b+n+j & n+j & b+n+j \\ \hline
        \multirow{4}{*}{SRResNet~\cite{ledig2017photo}} & None    & 23.21  & 22.70  & 21.59  & 21.44  & 22.24  & 22.05  & 18.25  & 18.43  & 20.42  & 20.10  \\ 
        ~ & Simple-Align~\cite{wang2024navigating}                   & 23.71  & 23.10  & 22.08  & 21.83  & 22.57  & 22.29  & 18.93  & 18.99  & 20.78  & \textbf{\textcolor{red}{20.29}}  \\ 
        ~ & Explicit Adaptive Dropout & \underline{\textcolor{blue}{23.71}} & \textbf{\textcolor{red}{23.10}} & \underline{\textcolor{blue}{22.09}} & \textbf{\textcolor{red}{21.84}} & \underline{\textcolor{blue}{22.59}} & \underline{\textcolor{blue}{22.31}} & \underline{\textcolor{blue}{18.95}} & \underline{\textcolor{blue}{19.04}} & \underline{\textcolor{blue}{20.79}} & \textbf{\textcolor{red}{20.29}} \\
        ~ & Implicit Adaptive Dropout & \textbf{\textcolor{red}{23.74}} & \textbf{\textcolor{red}{23.10}} & \textbf{\textcolor{red}{22.13}} & \textbf{\textcolor{red}{21.84}} & \textbf{\textcolor{red}{22.60}} & \textbf{\textcolor{red}{22.32}} & \textbf{\textcolor{red}{19.07}} & \textbf{\textcolor{red}{19.10}} & \textbf{\textcolor{red}{20.81}} & \textcolor{black}{20.27} \\ \hline
        \multirow{4}{*}{RRDB~\cite{zhang2018image}} & None    & 23.48  & 22.80  & 21.88  & 21.59  & 22.44  & 22.16  & 18.42  & 18.45  & 20.74  & 20.25  \\ 
        ~ & Simple-Align~\cite{wang2024navigating}                   & 23.85  & 23.06  & 22.22  & 21.85  & 22.67  & 22.36  & 19.00  & 19.02  & \textbf{\textcolor{red}{21.00}}  & 20.40  \\ 
        ~ & Explicit Adaptive Dropout & \textbf{\textcolor{red}{23.85}} & \underline{\textcolor{blue}{23.12}} & \underline{\textcolor{blue}{22.24}} & \underline{\textcolor{blue}{21.87}} & \textbf{\textcolor{red}{22.70}} & \textbf{\textcolor{red}{22.41}} & \underline{\textcolor{blue}{19.05}} & \underline{\textcolor{blue}{19.08}} & \underline{\textcolor{blue}{20.94}} & \textbf{\textcolor{red}{20.41}} \\ 
        ~ & Implicit Adaptive Dropout & \underline{\textcolor{blue}{23.87}} & \textbf{\textcolor{red}{23.10}} & \textbf{\textcolor{red}{22.28}} & \textbf{\textcolor{red}{21.90}} & \underline{\textcolor{blue}{22.68}} & \underline{\textcolor{blue}{22.40}} & \textbf{\textcolor{red}{19.06}} & \textbf{\textcolor{red}{19.12}} & \textbf{\textcolor{red}{20.94}} & \underline{\textcolor{blue}{20.40}} \\ \hline
        \multirow{4}{*}{SwinIR~\cite{liang2021swinir}} & None      & 23.67  & 22.99  & 22.11  & 21.82  & 22.61  & 22.34  & 18.79  & 18.80  & 20.98  & 20.45  \\ 
        ~ & Simple-Align~\cite{wang2024navigating}                   & \underline{\textcolor{blue}{23.80}}  & 23.09  & \textbf{\textcolor{red}{22.33}}  & 21.90  &  \underline{\textcolor{blue}{22.76}}  & 22.39  & \textbf{\textcolor{red}{19.02}}  & \underline{\textcolor{blue}{19.03}}  & \underline{\textcolor{blue}{21.12}}  & 20.53  \\ 
        ~ & Explicit Adaptive Dropout & \textbf{\textcolor{red}{23.82}} & \textbf{\textcolor{red}{23.18}} & \underline{\textcolor{blue}{22.30}} & \underline{\textcolor{blue}{22.19}} & \textbf{\textcolor{red}{22.78}} & \textbf{\textcolor{red}{22.50}} & \textcolor{black}{18.82} & \textcolor{black}{18.91} & \textbf{\textcolor{red}{21.15}} & \textbf{\textcolor{red}{20.57}} \\
       ~ & Implicit Adaptive Dropout & \textcolor{black}{23.76} & \underline{\textcolor{blue}{23.13}} & \textcolor{black}{22.23}  & \textbf{\textcolor{red}{22.19}} & \textcolor{black}{22.57} & \underline{\textcolor{blue}{22.39}} & \underline{\textcolor{blue}{18.87}} & \textbf{\textcolor{red}{19.10}} & \textcolor{black}{21.02} & \underline{\textcolor{blue}{20.56}} \\ \hline
    \end{tabular}}
  \end{center}

  \vskip -0.30cm
  \end{table*}

\subsection{About extensions on single-degradation tasks}
We tested our regularization method on three tasks: image deraining, image denoising, and image dehazing. We use Adaptive Dropout and set $w$ to $0.9$ in all blocks to simply verify the effectiveness of our method. The specific models, datasets, and results have been presented in the main text. Here, we display the visual results in~\figurename~\ref{fig:single}. It can be observed that the baseline fails to restore image quality well when encountering degradations and scenes inconsistent with training. In contrast, Adaptive Dropout helps these models generate more general representations to perform well on inconsistent degradations.

\begin{figure*}[t]
	\centering
	\includegraphics[width=1\linewidth]{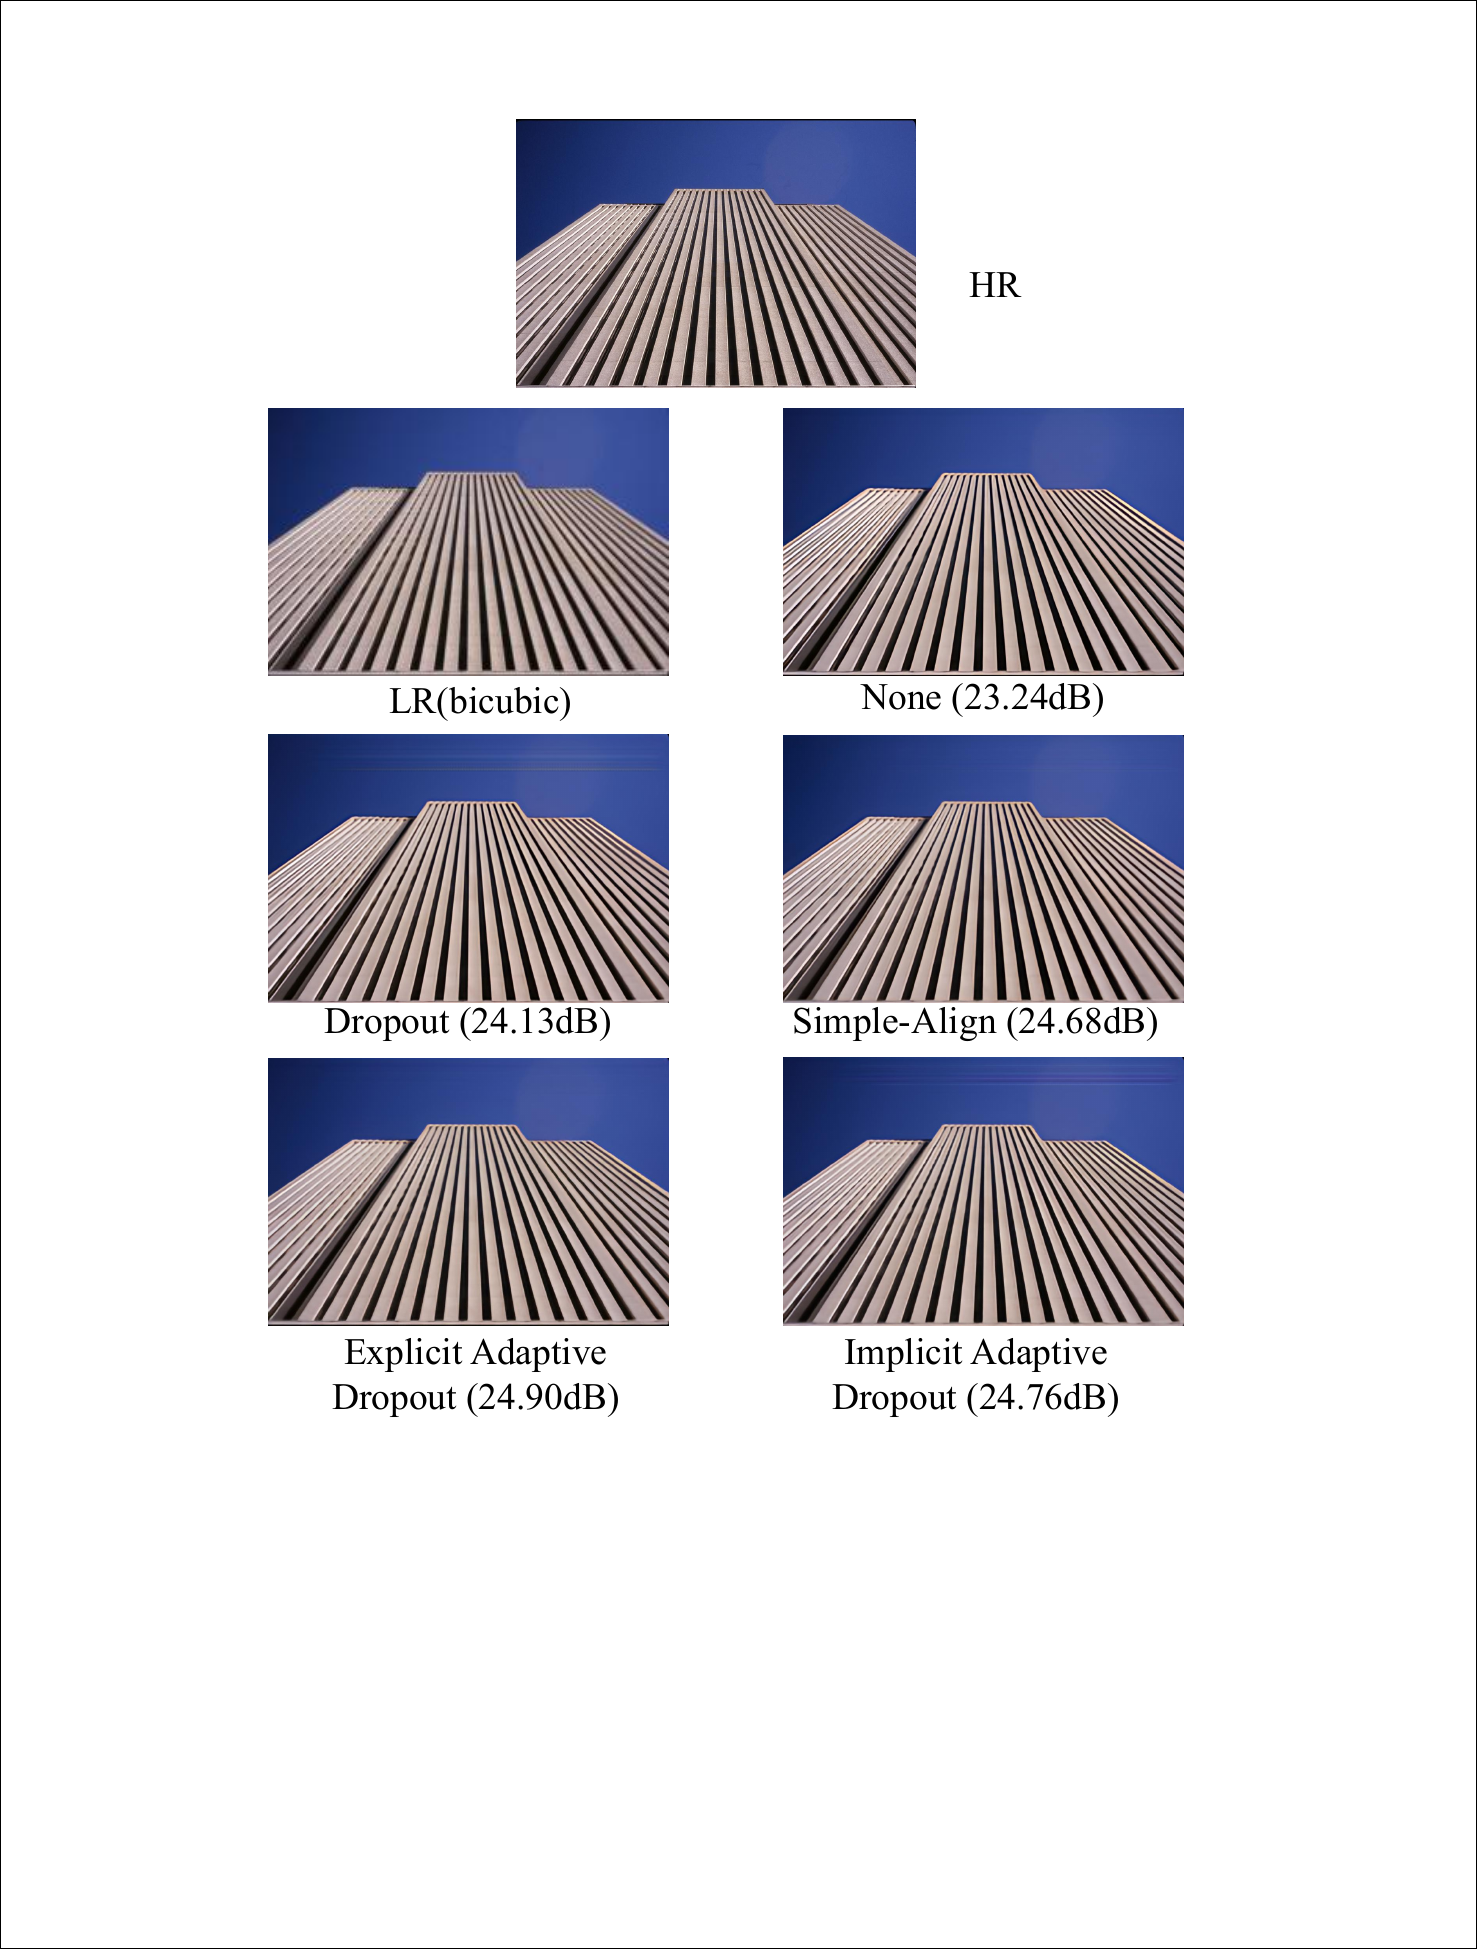}
    \vspace{-5mm}
	\caption{ \textbf{Visual comparison of our methods and past methods in “bicubic”.}}
	\label{fig:suppl_comparison_1}
\end{figure*}

\begin{figure*}[t]
	\centering
	\includegraphics[width=1\linewidth]{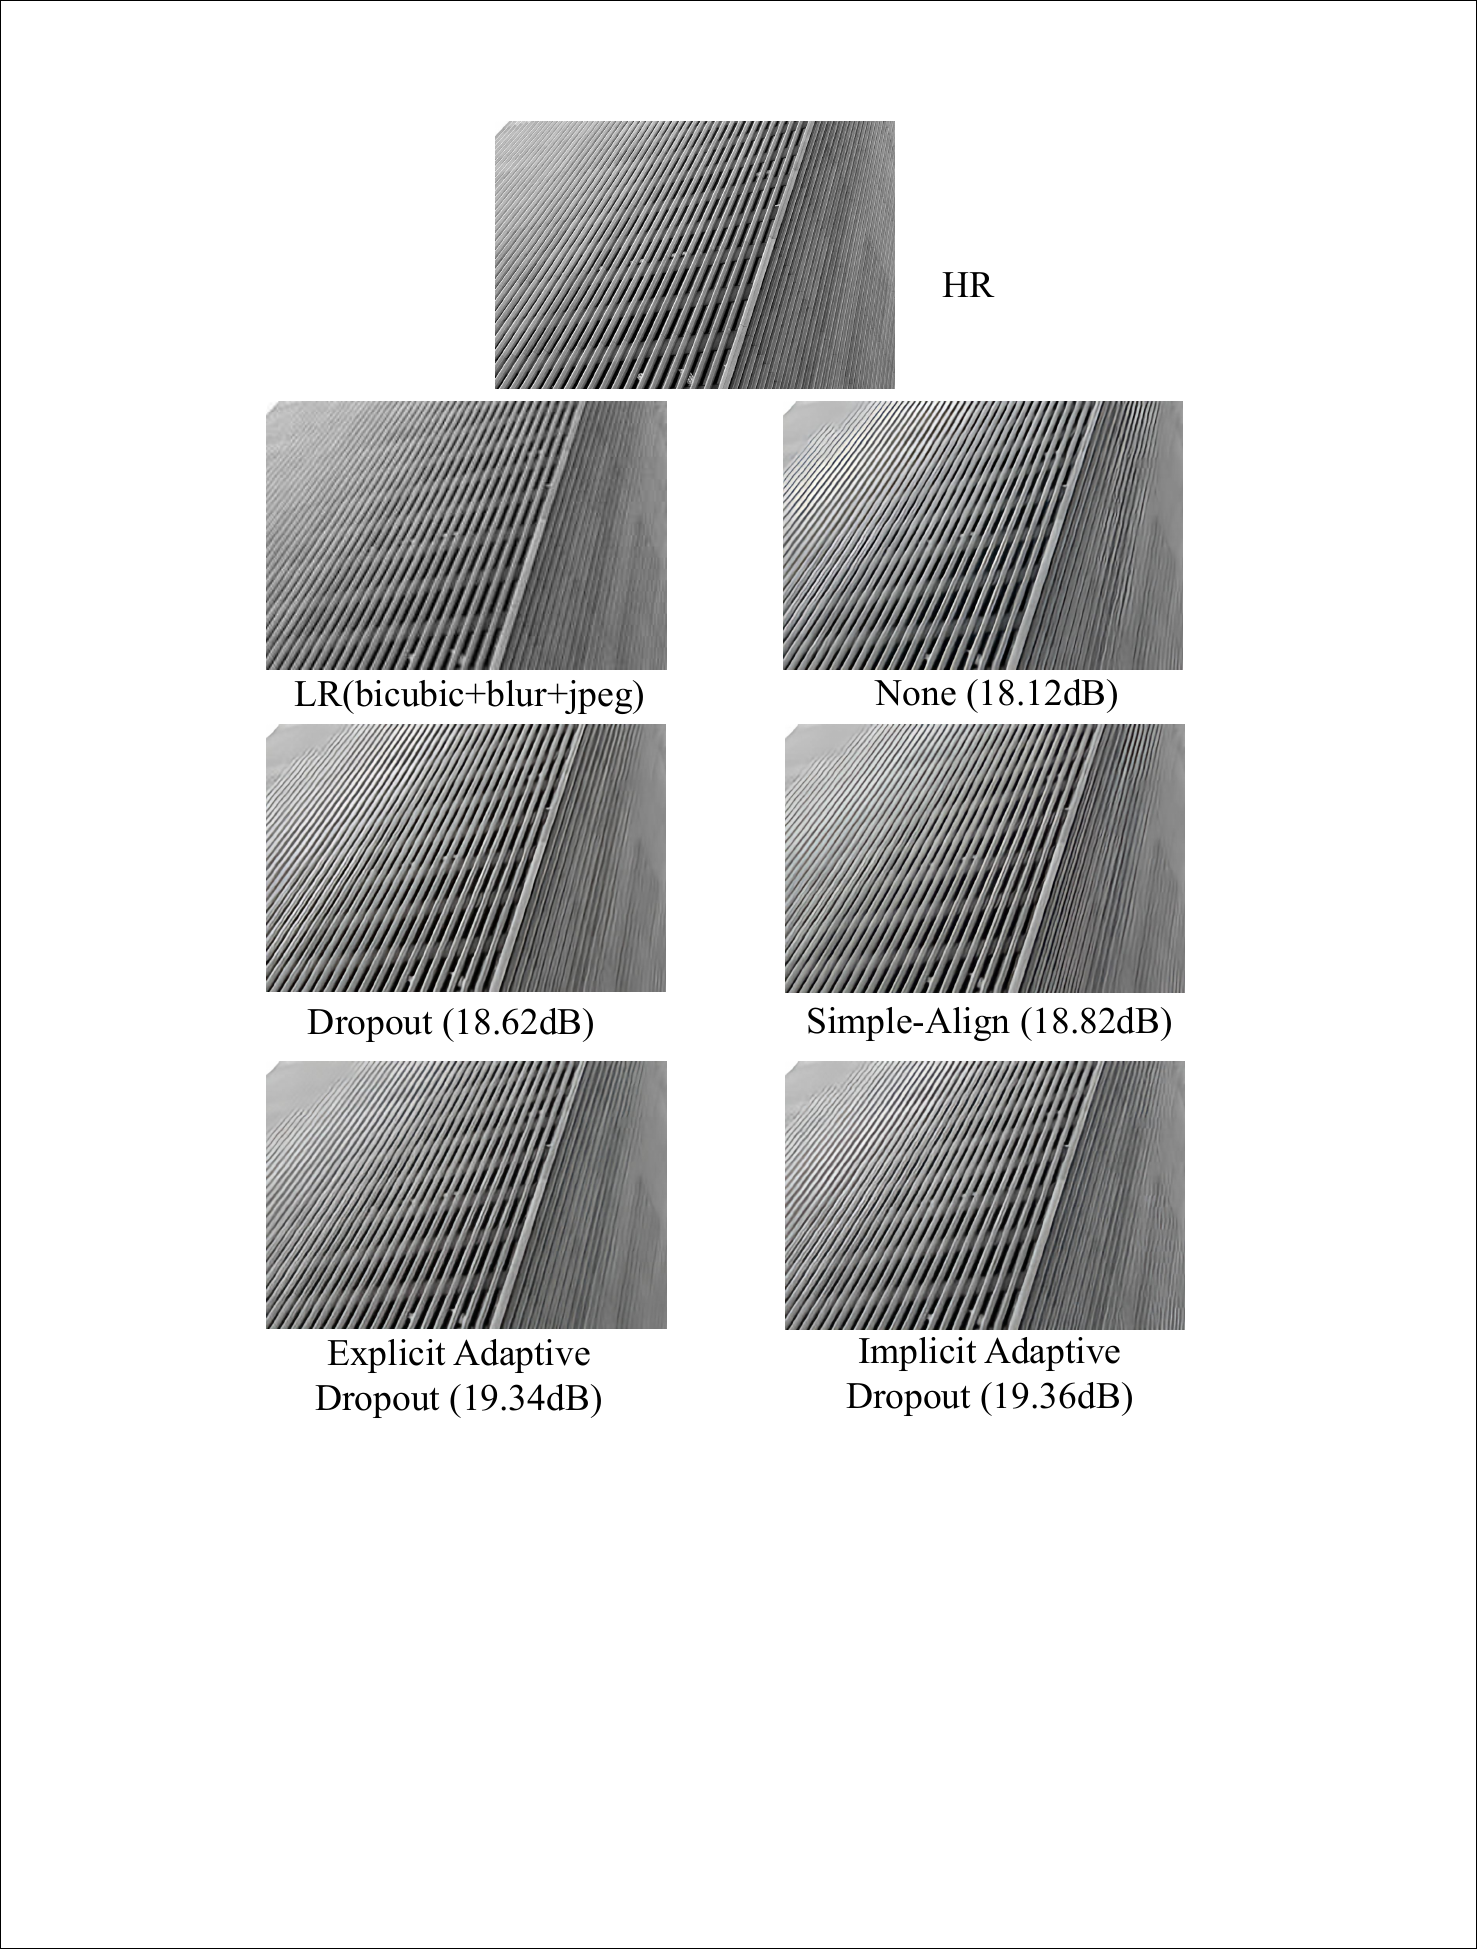}
    \vspace{-5mm}
	\caption{ \textbf{Visual comparison of our methods and past methods in “bicubic+blur+jpeg”.}}
	\label{fig:suppl_comparison_2}
\end{figure*}

\begin{figure*}[t]
	\centering
	\includegraphics[width=1\linewidth]{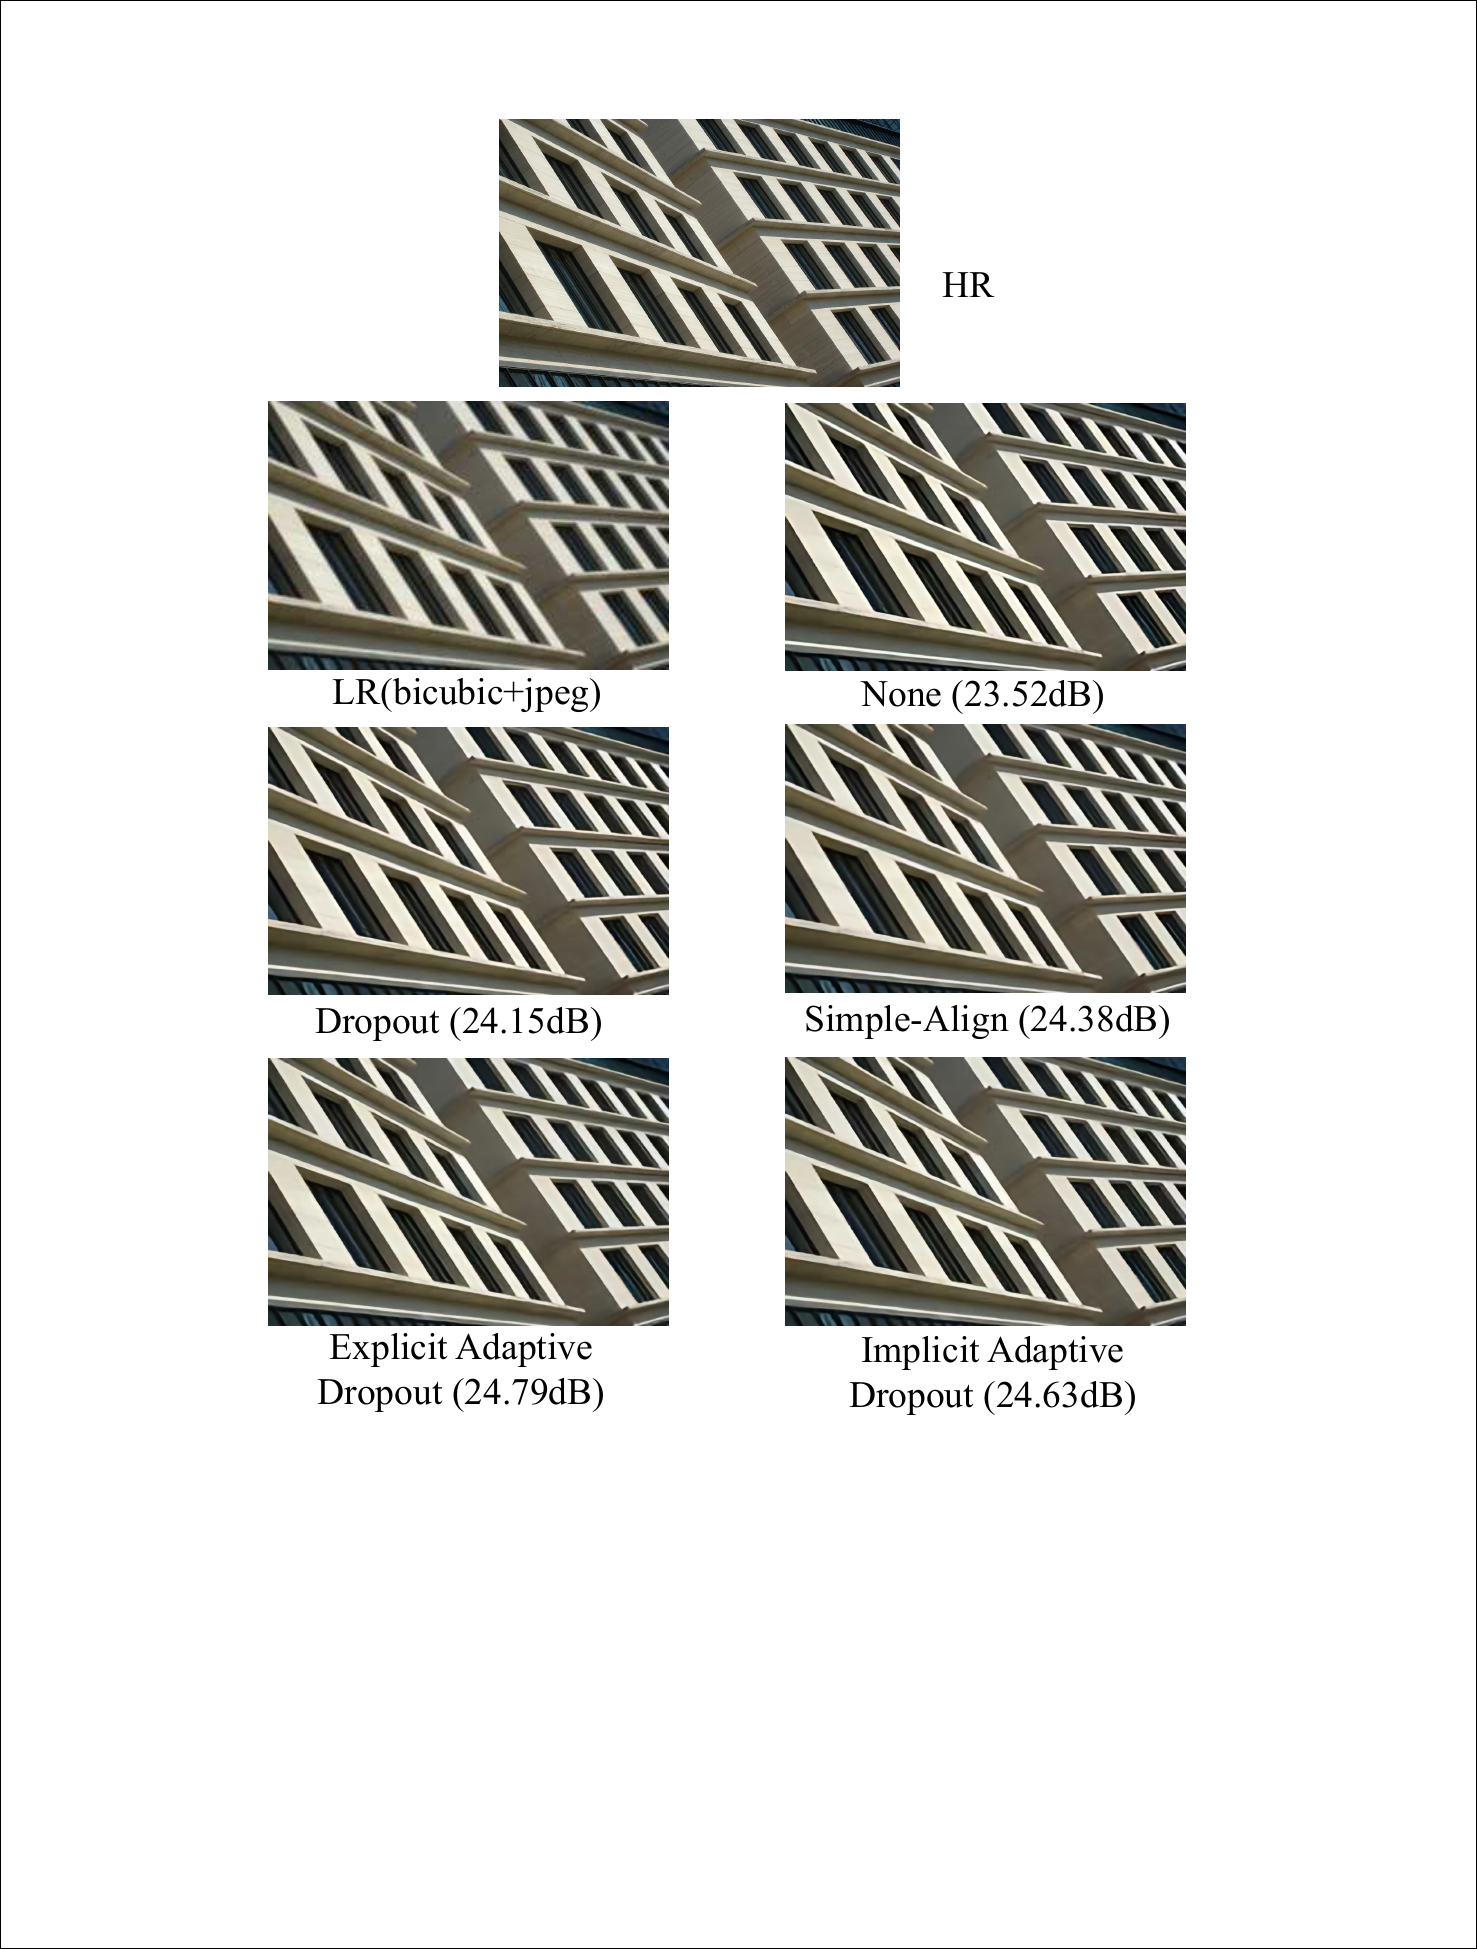}
    \vspace{-5mm}
	\caption{ \textbf{Visual comparison of our methods and past methods in “bicubic+jpeg”.}}
	\label{fig:suppl_comparison_3}
\end{figure*}

\begin{figure*}[t]
	\centering
	\includegraphics[width=1\linewidth]{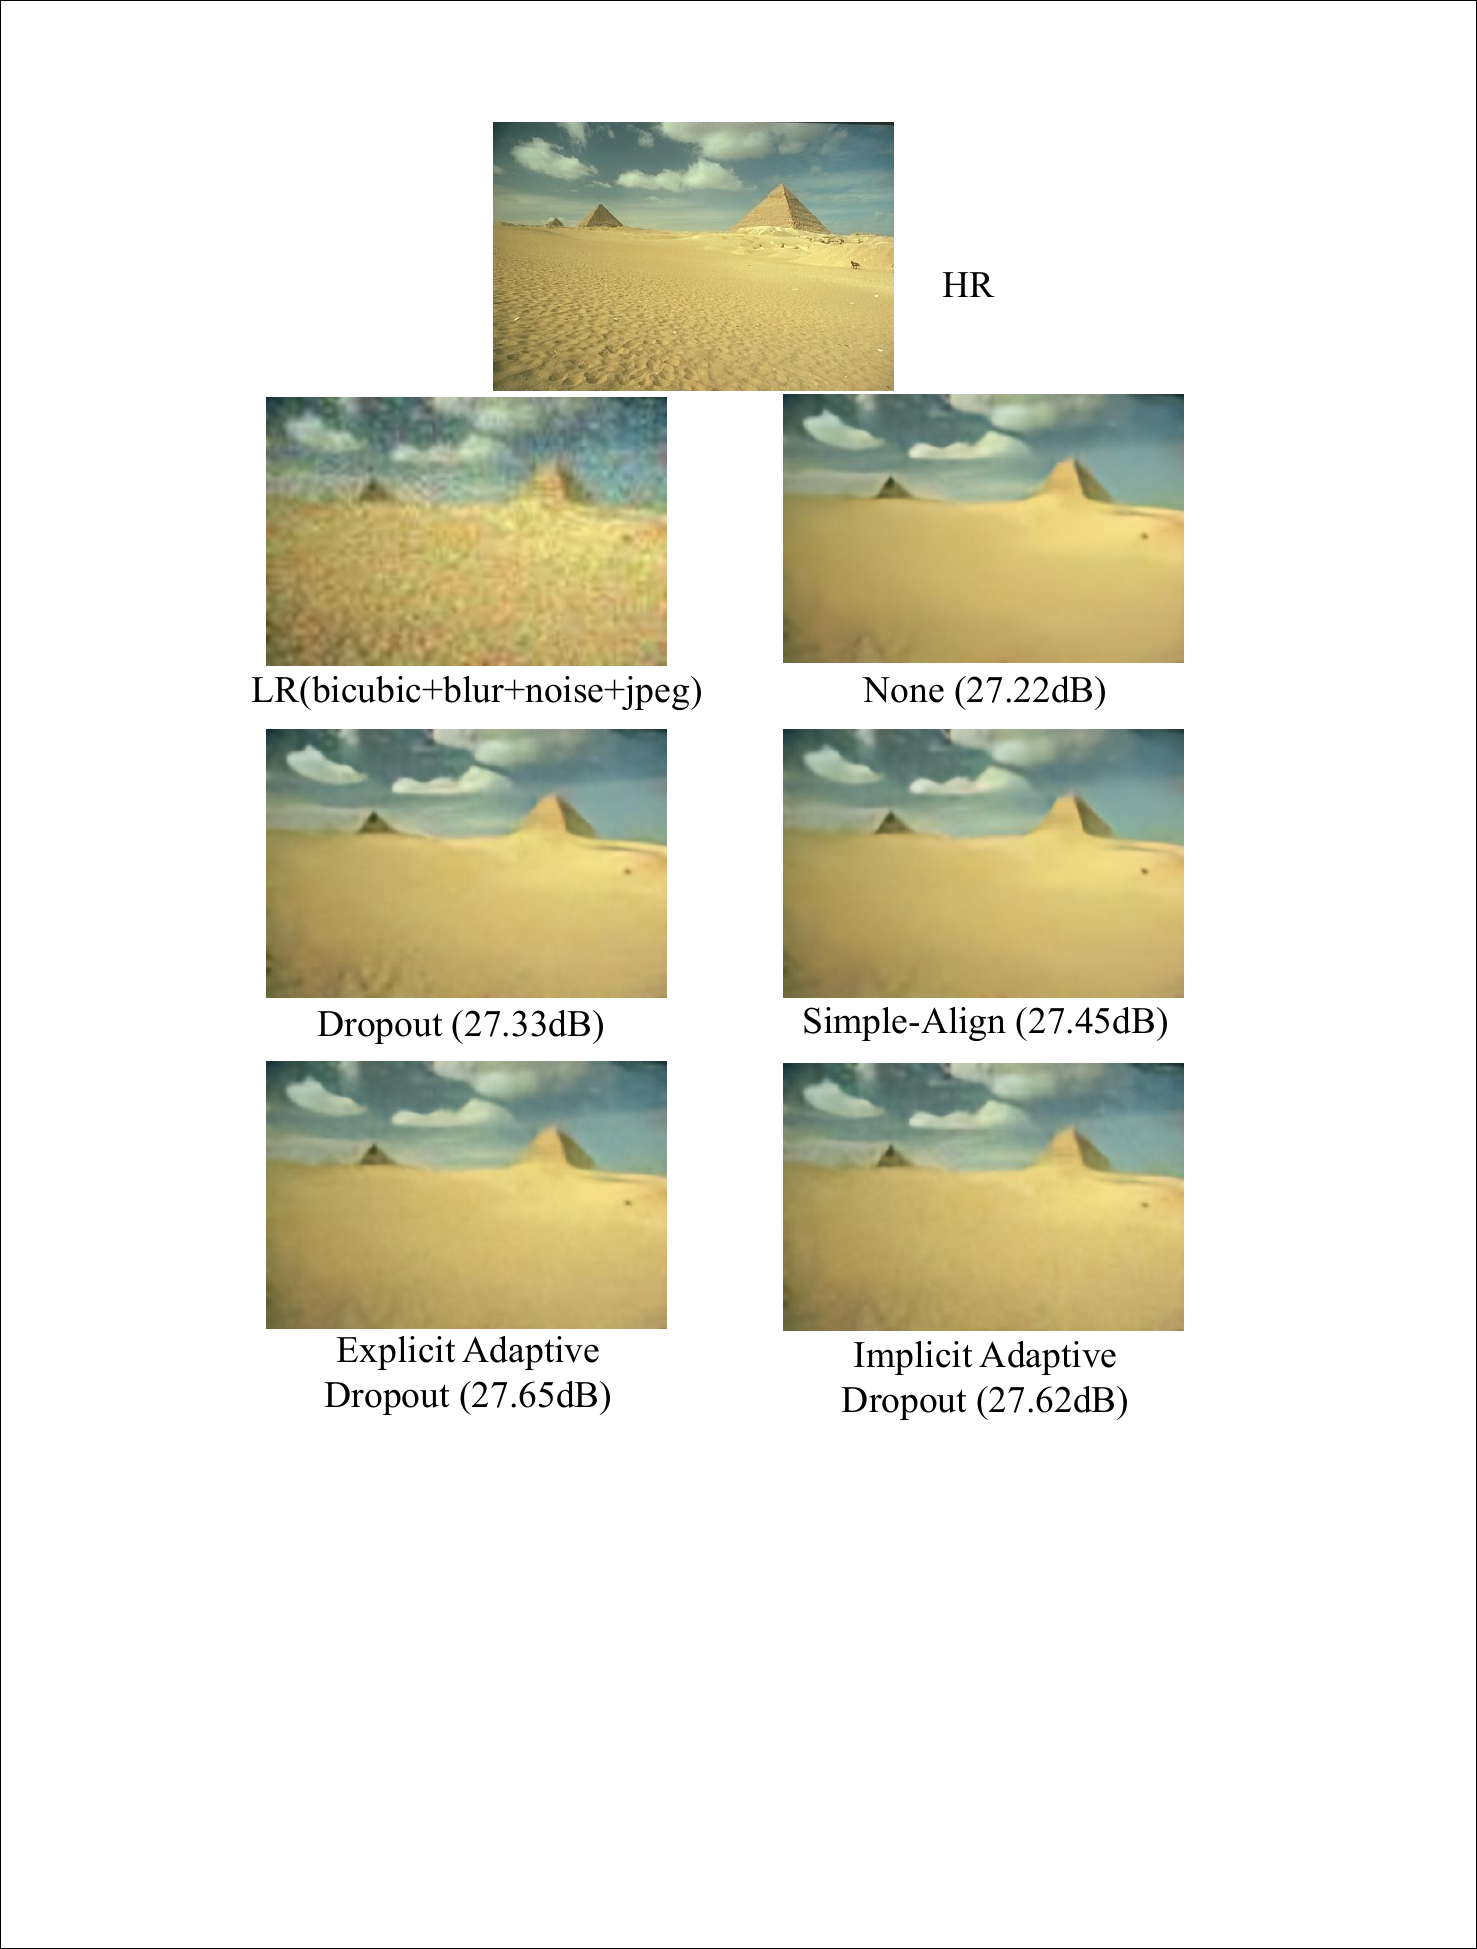}
    \vspace{-5mm}
	\caption{ \textbf{Visual comparison of our methods and past methods in “bicubic+blur+noise+jpeg”.}}
	\label{fig:suppl_comparison_4}
\end{figure*}
