# Supplementary material for: Adaptive Dropout: Unleashing Dropout across Layers for Generalizable Image Super-Resolution
Source: arXiv:2506.12738 source file (2025-06-15)
Supplement: Supplementary file 3 [file strategy_comparison.tex]

\begin{table}[h]
    \centering
    \small
  \setlength{\abovecaptionskip}{-0pt}
	\setlength{\belowcaptionskip}{-4pt}
	
     \caption{\textbf{The performance of SRResNet on Set5 and Set14 with different annealing strategies.} These annealing strategies are all for Explicit Adaptive Dropout and are explicitly adopted.}
     \label{tab:strategy}
    \begin{tabular}{cccc}
    \hline
         \multirow{2}{*}{dropout~format} &\multirow{2}{*}{training~strategy}  &\multicolumn{2}{c}{psnr} \\
         ~ & &Set5 &Set14 \\ \hline
         \multirow{4}{*}{standard dropout} &None &24.33 &22.45\\
         ~ &linear annealing &24.55 &22.83 \\
         ~ &layer-wise annealing &\textbf{24.89} &\textbf{23.01} \\
         ~ &linear+layer-wise &24.81 &22.94 \\ \hline
         \multirow{4}{*}{adaptive dropout} &None &25.89 &23.36\\
         ~ &linear annealing &25.85 &23.26\\
         ~ &layer-wise annealing &\textbf{26.07} &\textbf{23.46}\\
         ~ &linear+layer-wise &25.91 &23.32 \\ \hline
    \end{tabular}
    \vskip -0.10cm
\end{table}
