# Supplementary material for: Adaptive Dropout: Unleashing Dropout across Layers for Generalizable Image Super-Resolution
Source: arXiv:2506.12738 source file (2025-06-15)
Supplement: Supplementary file 5 [file w_format.tex]

\begin{table*}[h]
    \centering
    \small
  \setlength{\abovecaptionskip}{-0pt}
	\setlength{\belowcaptionskip}{-4pt}
	
     \caption{\textbf{The performance of SRResNet with different formats of $w$.} $nth~block$ means that before $nth$ block, we use $value~w$ and after $nth$ block, we use $vector~w$.}
     \label{tab:w_format}
    \begin{tabular}{ccccccc}
    \hline
         \multirow{2}{*}{nth block} &\multicolumn{6}{c}{model performance} \\
         ~ &Set5 &Set14 &BSD100 &Manga109 &Urban100 &average\\ \hline
         0 &24.61 &22.55 &23.00 &19.13 &20.67 &21.99\\
         4 &24.58 &22.56 &22.94 &19.23 &20.69 &22.00\\
         8 &24.55 &22.50 &22.94 &19.29 &20.81 &\textbf{22.09}\\
         12 &24.37 &22.40 &22.75 &19.40 &20.78 &21.94\\
         16 &24.28 &22.36 &22.86 &19.44 &21.02 &21.98\\ \hline
    \end{tabular}
    \vskip -0.10cm
\end{table*}
