# Supplementary material for: Adaptive Dropout: Unleashing Dropout across Layers for Generalizable Image Super-Resolution
Source: arXiv:2506.12738 source file (2025-06-15)
Supplement: Supplementary file 6 [file w_position.tex]

\begin{table}[h]
    \centering
    \small
  \setlength{\abovecaptionskip}{-0pt}
	\setlength{\belowcaptionskip}{-4pt}
	
     \caption{\textbf{The average performance of SRResNet on the five synthetic datasets.} We only calculate the average on the first four degradations(clean, noise, blur, jpeg), considering they best reflect the network's generalization capability. $plan~A$ is using $value~w$ for shallow layers and using $vector~w$ for deep layers. $plan~B$ is the opposite one.}
     \label{tab:w_position}
    \begin{tabular}{ccccccc}
    \hline
         postion &average performance \\ \hline
         plan A &\textbf{22.09} \\
         plan B &22.01 \\ \hline
    \end{tabular}
    \vskip -0.10cm
\end{table}
